# Supplementary material for: Electric field induced gelation in aqueous nanoclay suspensions
Source: arXiv:1807.08581 ancillary file (2018-07-23)
Supplement: Supplementary file 1 [file SI_Final.pdf]

# Electric field induced gelation in aqueous nanoclay suspensions

*Paramesh Gadige and Ranjini Bandyopadhyay* ∗

Soft Condensed Matter Group, Raman Research Institute,

C. V. Raman Avenue, Sadashivanagar, Bangalore 560 080, INDIA

∗ Electronic address: ranjini@rri.res.in

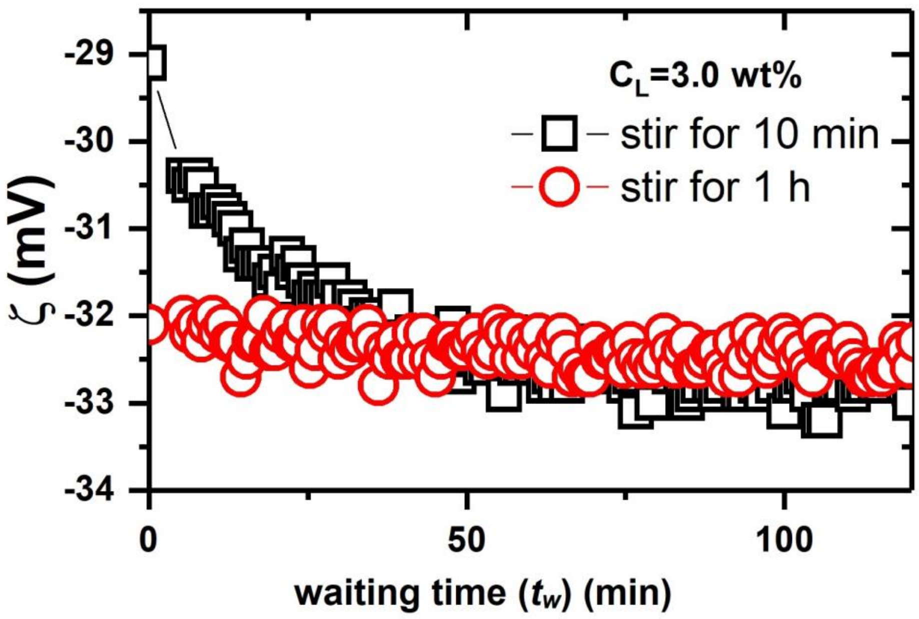


FIG. S1: Dependence of Zeta potential of Laponite suspensions on initial stirring duration.

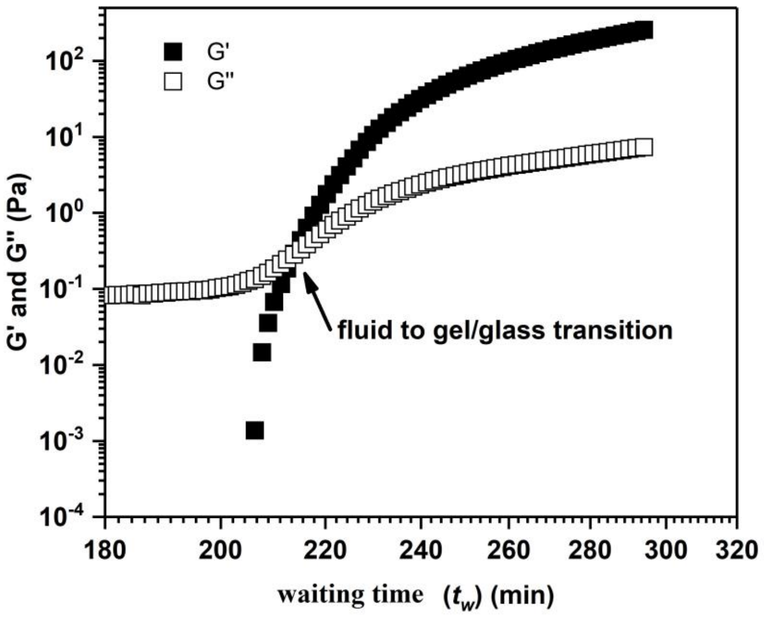


FIG. S2: Spontaneous evolution of $G'$ and $G''$ of Laponite suspensions with increasing waiting time ($t_w$).

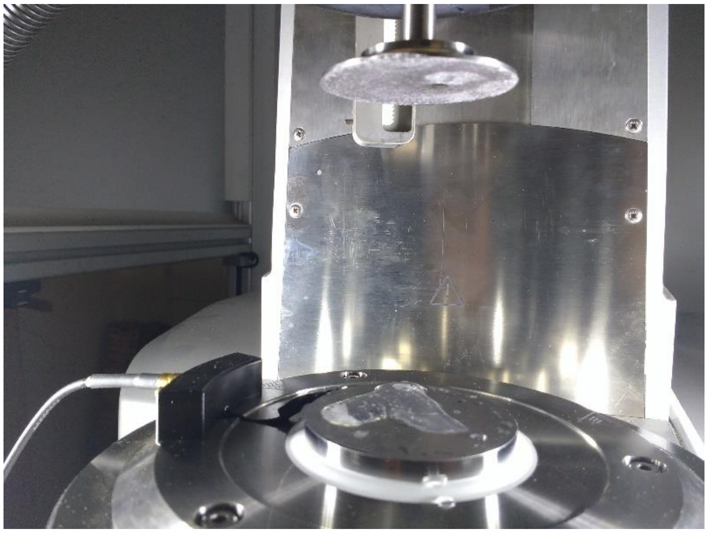

Fig. S3. The top plate of the rheometer was connected to the positive voltage supply and the bottom plate was connected to the negative electrode. The clay gel formed over the surface of the top plate (+ve electrode) can be seen in the figure as a thick (viscoelastic) white residue that sticks to the surface after few minutes of applying voltage 20 V between 1 mm gap (in the rheo-dielectric sample cell). The bottom plate, in contrast, shows no gel formation. Only a film of watery liquid is visible on the bottom surface.
